# Supplementary material for: Intersection Information based on Common Randomness
Source: arXiv:1310.1538 source file (2015-06-10)
Supplement: Supplementary file 1 [file appendix.tex]

%%%%%%%%%%%%%%%%%%%%%%%%%%%%%%%%%%%%%%%%%%%%%%%%%%%%%%%%%%%%%%%%%%%%%%%%%%
\part*{Appendix}
\appendix
%%%%%%%%%%%%%%%%%%%%%%%%%%%%%%%%%%%%%%%%%%%%%%%%%%%%%%%%%%%%%%%%%%%%%%%%%%
\section{Algorithm for Computing Common Random Variable}
\label{appendix:crv}
Given $n$ random variables $X_1,\ldots,X_n$, the common random variable $X_1 \wedge \cdots \wedge X_n$ is computed by steps 1--3 in Appendix~\ref{appendix:computingIcrv}.

\section{Algorithm for Computing $\Iw$}
\label{appendix:computingIcrv}
\begin{enumerate}
    \item For each $X_i$ for $i=1,\ldots,n$, take its states $x_i$ and place them as nodes on a graph.  At the end of this process there will be $\sum_{i=1}^n |X_i|$ nodes on the graph.

    \item For each pair of RVs $X_i$, $X_j$ ($i \not= j$), draw an undirected edge connecting nodes $x_i$ and $x_j$ if $\Prob{x_i, x_j} > 0$.  At the end of this process the undirected graph will consist of $k$ connected components $1 \leq k \leq \min_i |X_i|$.  Denote these $k$ disjoint components as $\mathbf{c_1, \ldots, c_k}$.

    \item Each connected component of the graph constitutes a
distinct state of the common random variable $Q$, i.e., $|Q|=k$.  Denote the states of the common random variable $Q$ by $q_1, \ldots, q_k$.

    \item Construct the joint probability distribution $\Prob{Q,Y}$ as follows.  For every state $(q_i, y) \in Q\times Y$, the joint probability is created by summing over the entries of $\Prob{x_1, \ldots, x_n, y}$ in component $i$.  More precisely,
\begin{equation*}
 \Prob{Q = q_i, Y = y} = \sum_{x_1,\ldots,x_n} \Prob{x_1, \ldots, x_n, y} \qquad \textnormal{if }\{x_1, \ldots, x_n\} \subseteq \mathbf{c_i} \; .
\end{equation*}

    \item Using $\Prob{Q,Y}$, compute $\Iwe{X_1, \ldots, X_n}{Y}$
simply by computing the Shannon mutual information between $Q$ and
$Y$, i.e., $\info{Q}{Y} = \DKL{ \Prob{Q,Y} }{ \Prob{Q} \Prob{Y} }$.

\end{enumerate}

\section{Lemmas and Proofs}

\subsection{Lemmas on Desired Properties}
\label{app:prop}

\begin{lem}\label{lem:LBwedge}
If \LB holds, then
$\Icape{ X_1, \ldots, X_n }{Y} \geq \Infor{X_1 \wedge \cdots \wedge X_n}{Y}$.
\end{lem}

\begin{proof}
Assume that \LB holds. By definition, $X_1 \wedge \cdots
\wedge X_n \preceq X_i$ for $i=1,\ldots,n$. So, by  \LB,
we immediately conclude that $\Icape{ X_1, \ldots, X_n }{Y} \geq
\Infor{X_1 \wedge \cdots \wedge X_n}{Y}$, which is the desired
result.
\end{proof}

For the converse, we need the following assumption:
\begin{itemize}
\item[\IM] If $X_1\preceq X_2$, then $\Infor{X_1}{Y}\leq\Infor{X_2}{Y}$.
\end{itemize}

\begin{lem}\label{lem:LBwedgeIM}
Suppose that \IM holds, and that
$\Icape{ X_1, \ldots, X_n }{Y} \geq \Infor{X_1 \wedge \cdots \wedge X_n}{Y}$.
Then \LB holds.
\end{lem}

\begin{proof}
Assume that $\Icape{ X_1, \ldots, X_n }{Y} \geq \Infor{X_1 \wedge
\cdots \wedge X_n}{Y}$. Let $Q\preceq X_i$ for $i=1,\ldots,n$.
Because $X_1 \wedge \cdots \wedge X_n$ is the largest (informationally
richest) random variable that is informationally poorer than $X_i$
for $i=1,\ldots,n$, it follows that $Q \preceq X_1 \wedge \cdots
\wedge X_n$. Therefore, by \IM, $\Infor{X_1 \wedge \cdots \wedge
X_n}{Y} \geq \Infor{Q}{Y}$. Hence, $\Icape{X_1,\ldots,X_n}{Y} \geq
\Infor{Q}{Y}$ also, which completes the proof.
\end{proof}

\textbf{Remark:} Assumption \IM is satisfied by zero-error information and Shannon mutual information.

\begin{lem} \label{lem:condIcap}
Given $\Icap$, $X_1,\ldots,X_n$, $Y$, and $Z$, consider the
conditional intersection information
\[
\Icap\!\left( X_1,\ldots,X_n \: Z \middle| Y \right)
= \Icape{X_1,\ldots,X_n}{Y\vee Z}-\Icape{X_1,\ldots,X_n}{Y}.
\]
Suppose that \GP, \Eq, and \TM hold. Then, the following properties hold:
\begin{itemize}
\item $\Icap\!\left( X_1,\ldots,X_n \: Z \middle| Y \right)\geq 0$.
\item $\Icap\!\left( X_1,\ldots,X_n \: Z \middle| Y \right)=\Icape{X_1,\ldots,X_n}{Z}$ if $Y$ is a constant.
\end{itemize}
\end{lem}

\begin{proof}
We have $Y\preceq Y\vee Z$. Therefore, by \TM, it
immediately follows that
$\Icap\!\left( X_1,\ldots,X_n \: Z \middle| Y \right)\geq 0$.

Next, suppose that $Y$ is a constant. Then $Y\preceq Z$, and hence $Y\vee Z\cong Z$. By
\Eq, $\Icape{X_1,\ldots,X_n}{Y\vee Z}=\Icape{X_1,\ldots,X_n}{Z}$.
Moreover, by \GP, $\Icape{X_1,\ldots,X_n}{Y}=0$. Thus,
$\Icap\!\left( X_1,\ldots,X_n \: Z \middle| Y
\right)=\Icape{X_1,\ldots,X_n}{Z}$ as desired.
\end{proof}

\subsection{Properties of $\Iw^0$}
\label{app:Iw0}

\begin{lem}\label{lem:Iw0prop0}
The measure of intersection information $\Iw^0\!\left(X_1,\ldots,X_n \: Y \right)$ satisfies
\GP,
\Eq,
\TM,
\Mzero, and
\Szero, but not
\LPzero.
\end{lem}

\begin{proof}
\GP: The inequality
$\Iw^0\!\left( X_1,\ldots,X_n : Y \right) \geq 0$
follows immediately from the identity
$\Iw^0\!\left( X_1,\ldots,X_n : Y \right) = \ent{ X_1 \wedge \cdots \wedge X_n \wedge Y } $
and the nonnegativity of $\ent{\cdot}$. Next,
if $Y$ is a constant, then by the generalized absorption law,
$X_1 \wedge \cdots \wedge X_n \wedge Y \cong Y$. Thus, by the invariance of $\ent{\cdot}$ (Lemma~\ref{lem:H}(a)),
$\ent{X_1 \wedge \cdots \wedge X_n \wedge Y} = \ent{Y}=0$.

\Eq: Consider $X_1 \wedge \cdots \wedge X_n \wedge Y$.
The equivalence class (with respect to $\cong$) in which this
random variable resides is closed under
substitution of $X_i$ (for $i=1,\ldots,n$) or $Y$ by an
informationally equivalent random variable. Hence, because
$\Iw^0\!\left( X_1,\ldots,X_n : Y \right) = \ent{ X_1 \wedge \cdots
\wedge X_n \wedge Y }$ and $\ent{\cdot}$ is invariant over the
equivalence class of random variables that are informationally
equivalent to $X_1 \wedge \cdots \wedge X_n \wedge Y$ (by Lemma~\ref{lem:H}(a)), the desired
result holds.

\TM: Suppose that $Y\preceq Z$. Then,
$X_1 \wedge \cdots \wedge X_n \wedge Y \preceq
X_1 \wedge \cdots \wedge X_n \wedge Z$.
Then, we have
\begin{align*}
\Iw^0\!\left( X_1,\ldots,X_n : Y \right)
&= \ent{X_1 \wedge \cdots \wedge X_n \wedge Y} \\
&\leq \ent{X_1 \wedge \cdots \wedge X_n \wedge Z}
\quad\mbox{by monotonicity of $\ent{\cdot}$ (Lemma~\ref{lem:H}(b))} \\
&= \Iw^0\!\left( X_1,\ldots,X_n : Z \right),
\end{align*}
as desired.

\Mzero:
By the generalized absorption law,
$X_1 \wedge \cdots \wedge X_n \wedge W \wedge Y \preceq
X_1 \wedge \cdots \wedge X_n \wedge Y$.
Hence,
\begin{align*}
\Iw^0\!\left( X_1,\ldots,X_n,W : Y \right)
&= \ent{X_1 \wedge \cdots \wedge X_n \wedge W \wedge Y} \\
&\leq \ent{X_1 \wedge \cdots \wedge X_n \wedge Y}
\quad\mbox{by monotonicity of $\ent{\cdot}$ (Lemma~\ref{lem:H}(b))} \\
&= \Iw^0\!\left( X_1,\ldots,X_n : Y \right),
\end{align*}
as desired.

Next, suppose that there exists $Z\in\{X_1,\ldots,X_n\}$ such that
$Z\preceq W$. Then, by the generalized absorption law,
$X_1 \wedge \cdots \wedge X_n \wedge W \wedge Y \cong
X_1 \wedge \cdots \wedge X_n \wedge Y$.
Hence,
\begin{align*}
\Iw^0\!\left( X_1,\ldots,X_n,W : Y \right)
&= \ent{X_1 \wedge \cdots \wedge X_n \wedge W \wedge Y} \\
&= \ent{X_1 \wedge \cdots \wedge X_n \wedge Y}
\quad\mbox{by invariance of $\ent{\cdot}$ (Lemma~\ref{lem:H}(a))} \\
&= \Iw^0\!\left( X_1,\ldots,X_n : y \right),
\end{align*}
as desired.

\Szero:
By the commutativity law, $X_1 \wedge \cdots \wedge X_n \wedge Y $
is invariant (with respect to $\cong$) under reordering of $X_1,\ldots,X_n$.
Hence, the desired result follows immediately from the identity
$\Iw^0\!\left( X_1,\ldots,X_n : Y \right)
= \ent{ X_1 \wedge \cdots \wedge X_n \wedge Y }$ and the
invariance of $\ent{\cdot}$ (Lemma~\ref{lem:H}(a)).

\LPzero:
For $\Iw^0$, \LPzero relative to zero-error information can be written as
\begin{equation}
\ent{X_1\wedge X_2\wedge Y} \geq \ent{X_1\wedge Y} + \ent{X_2\wedge Y} - \ent{(X_1\vee X_2)\wedge Y}.
\label{eqn:LP0}
\end{equation}
However, this inequality does not hold in general. To see this, suppose that it does hold for arbitrary $X_1$, $X_2$, and $Y$. Note that $(X_1\vee X_2)\wedge Y \preceq Y$, which implies that $\ent{(X_1\vee X_2)\wedge Y} \leq \ent{Y}$ (by monotonicity of $\ent{\cdot}$). Hence, the inequality (\ref{eqn:LP0}) implies that
\[
\ent{X_1\wedge X_2\wedge Y} \geq \ent{X_1\wedge Y} + \ent{X_2\wedge Y} - \ent{Y}.
\]
Rewriting this, we get
\[
\ent{X_1\wedge Y} + \ent{Y\wedge X_2} \leq \ent{X_1\wedge Y\wedge X_2} + \ent{Y}.
\]
But this is the supermodularity law for common information, which is known to be false in general; see \cite{li11}, Section 5.4.

\end{proof}

\begin{lem}\label{lem:Iw0propInfor}
With respect to zero-error information, the measure of intersection information $\Iw^0\!\left(X_1,\ldots,X_n \: Y \right)$ satisfies
\LB,
\SR, and
\Id.
\end{lem}

\begin{proof}
\LB:
Suppose that $Q\preceq X_i$ for $i=1,\ldots,n$.
Because $X_1 \wedge \cdots \wedge X_n$ is the largest (informationally
richest) random variable that is informationally poorer than $X_i$
for $i=1,\ldots,n$, it follows that $Q \preceq X_1 \wedge \cdots
\wedge X_n$. This implies that
$X_1 \wedge \cdots \wedge X_n \wedge Y \succeq Q \wedge Y$.
Therefore,
\begin{align*}
\Iw^0\!\left(X_1, \ldots, X_n : Y \right)
 &=  \ent{ X_1 \wedge \cdots \wedge X_n \wedge Y } \\
 &\geq  \ent{ Q \wedge Y }\quad \mbox{by monotonicity of $\ent{\cdot}$ (Lemma~\ref{lem:H}(b))} \\
 &= \infozero{Q}{Y},
\end{align*}
as desired.

\SR:
We have $\Iw^0( X_1 : Y ) = \ent{ X_1 \wedge Y } = \infozero{X_1}{Y}$.

\Id:
By the associative and absorption laws, we have $X \wedge Y \wedge (X\vee Y) \cong X\wedge Y$.
Thus,
\begin{align*}
\Iw^0\!\left(X,Y : X\vee Y \right)
 &= \ent{ X \wedge Y \wedge (X\vee Y) } \\
 &= \ent{ X \wedge Y} \quad\mbox{by invariance of $\ent{\cdot}$ (Lemma~\ref{lem:H}(a))} \\
 &= \infozero{X}{Y},
\end{align*}
as desired.

\end{proof}

\begin{lem}\label{lem:Iw0prop1}
The measure of intersection information $\Iw^0\!\left(X_1,\ldots,X_n \: Y \right)$ satisfies \Mone and \Sone, but not \LPone. \end{lem}

\begin{proof}
\Mone:
The desired inequality is identical to \Mzero,
so it remains to prove the sufficient condition for equality. Suppose that there exists $Z\in\{X_1,\ldots,X_n,Y\}$ such that
$Z\preceq W$. Then, by the generalized absorption law,
$X_1 \wedge \cdots \wedge X_n \wedge W \wedge Y \cong
X_1 \wedge \cdots \wedge X_n \wedge Z$.
Hence,
\begin{align*}
\Iw^0\!\left( X_1,\ldots,X_n,W : Y \right)
&= \ent{X_1 \wedge \cdots \wedge X_n \wedge W \wedge Y} \\
&= \ent{X_1 \wedge \cdots \wedge X_n \wedge Z}
\quad\mbox{by invariance of $\ent{\cdot}$ (Lemma~\ref{lem:H}(a))} \\
&= \Iw^0\!\left( X_1,\ldots,X_n : Z \right),
\end{align*}
as desired.

\Sone:
By the commutativity law, $X_1 \wedge \cdots \wedge X_n \wedge Y $
is invariant (with respect to $\cong$) under reordering of $X_1,\ldots,X_n,Y$.
Hence, the desired result follows immediately from the identity
$\Iw^0\!\left( X_1,\ldots,X_n : Y \right)
= \ent{ X_1 \wedge \cdots \wedge X_n \wedge Y }$ and the
invariance of $\ent{\cdot}$ (Lemma~\ref{lem:H}(a)).

\LPone: This follows from not satisfying \LPzero.

\end{proof}

\subsection{Properties of $\Iw$}
\label{app:Iw}

\begin{lem}\label{lem:Iwprop0}
The measure of intersection information $\Iw\!\left(X_1,\ldots,X_n \: Y \right)$ satisfies
\GP,
\Eq,
\TM,
\Mzero, and
\Szero, but not
\LPzero.
\end{lem}

\begin{proof}
\GP: The inequality
$\Iw\!\left( X_1,\ldots,X_n : Y \right) \geq 0$
follows immediately from the identity
$\Iw\!\left( X_1,\ldots,X_n : Y \right) = \info{ X_1 \wedge \cdots \wedge X_n}{Y}$
and the nonnegativity of mutual information. Next, suppose that
$Y$ is a constant. Then $\ent{Y}=0$. Moreover,
$Y\preceq X_1 \wedge \cdots \wedge X_n$ by definition of $\wedge$.
Thus, by Lemma~\ref{lem:H}(c),  $\ent{Y|X_1 \wedge \cdots \wedge X_n}=0$, and
\begin{align*}
\Iw\!\left( X_1,\ldots,X_n : Y \right)
&= \info{X_1 \wedge \cdots \wedge X_n}{Y}  \\
&= \info{Y}{X_1 \wedge \cdots \wedge X_n} \\
&= \ent{Y} - \ent{Y|X_1 \wedge \cdots \wedge X_n}  \\
&= 0.
\end{align*}

\Eq: Consider $X_1 \wedge \cdots \wedge X_n \wedge Y$.
The equivalence class (with respect to $\cong$) in which this
random variable resides is closed under
substitution of $X_i$ (for $i=1,\ldots,n$) or $Y$ by an
informationally equivalent random variable. Hence, because
\begin{align*}
\Iw\!\left( X_1,\ldots,X_n : Y \right)
&= \ent{Y} - \ent{Y|X_1 \wedge \cdots \wedge X_n}  \\
&= \ent{X_1 \wedge \cdots \wedge X_n} - \ent{X_1 \wedge \cdots \wedge X_n|Y},
\end{align*}
by Lemma~\ref{lem:H}(a), the desired result holds.

\TM: Suppose that $Y\preceq Z$.
For simplicity, let $Q=X_1\wedge\cdots\wedge X_n$.  Then,
\begin{align*}
\Iw\!\left( X_1,\ldots,X_n : Y \right)
&= \ent{Q} - \ent{Q|Y} \\
&\leq \ent{Q} - \ent{Q|Z} \quad\mbox{by Lemma~\ref{lem:H}(b)} \\
&= \Iw\!\left( X_1,\ldots,X_n : Z \right),
\end{align*}
as desired.

\Mzero:
By definition of $\wedge$, we have
$X_1 \wedge \cdots \wedge X_n \wedge W \preceq X_1 \wedge \cdots \wedge X_n$.
Hence,
\begin{align*}
\Iw\!\left( X_1,\ldots,X_n,W : Y \right)
&= \ent{X_1 \wedge \cdots \wedge X_n \wedge W} - \ent{X_1 \wedge \cdots \wedge X_n \wedge W|Y} \\
&\leq \ent{X_1 \wedge \cdots \wedge X_n} - \ent{X_1 \wedge \cdots \wedge X_n|Y}
\quad\mbox{by Lemma~\ref{lem:H}(b)} \\
&= \Iw\!\left( X_1,\ldots,X_n : Y \right),
\end{align*}
as desired.

Next, suppose that there exists $Z\in\{X_1,\ldots,X_n\}$ such that
$Z\preceq W$. Then, by the algebraic laws of $\wedge$, we have
$X_1 \wedge \cdots \wedge X_n \wedge W \cong
X_1 \wedge \cdots \wedge X_n$.
Hence,
\begin{align*}
\Iw\!\left( X_1,\ldots,X_n,W : Y \right)
&= \ent{X_1 \wedge \cdots \wedge X_n \wedge W} - \ent{X_1 \wedge \cdots \wedge X_n \wedge W|Y} \\
&= \ent{X_1 \wedge \cdots \wedge X_n} - \ent{X_1 \wedge \cdots \wedge X_n|Y}
\quad\mbox{by Lemma~\ref{lem:H}(a)} \\
&= \Iw\!\left( X_1,\ldots,X_n : Y \right),
\end{align*}
as desired.

\Szero:
By the commutativity law, $X_1 \wedge \cdots \wedge X_n$
is invariant (with respect to $\cong$) under reordering of $X_1,\ldots,X_n$.
Hence, the desired result follows immediately from the identity
$\Iw\!\left( X_1,\ldots,X_n : Y \right)
= \ent{X_1 \wedge \cdots \wedge X_n} - \ent{X_1 \wedge \cdots \wedge X_n|Y}$
and Lemma~\ref{lem:H}(a).

\LPzero: A counterexample is provided by \textsc{ImperfectRdn} (\figref{fig:ImperfectRdn}).

\end{proof}

\begin{lem}\label{lem:IwpropInfor}
With respect to mutual information, the measure of intersection information $\Iw\left(X_1,\ldots,X_n \: Y \right)$ satisfies
\LB and \SR, but not \Id.
\end{lem}

\begin{proof}
\LB:
Suppose that $Q\preceq X_i$ for $i=1,\ldots,n$.
Because $X_1 \wedge \cdots \wedge X_n$ is the largest (informationally
richest) random variable that is informationally poorer than $X_i$
for $i=1,\ldots,n$, it follows that $Q \preceq X_1 \wedge \cdots
\wedge X_n$.
Therefore,
\begin{align*}
\Iw\!\left(X_1, \ldots, X_n : Y \right)
 &= \ent{X_1 \wedge \cdots \wedge X_n} - \ent{X_1 \wedge \cdots \wedge X_n|Y} \\
 &\geq \ent{Q} - \ent{Q|Y} \quad \mbox{by Lemma~\ref{lem:H}(b)} \\
 &= \info{Q}{Y},
\end{align*}
as desired.

\SR:
By definition, $\Iw( X_1 : Y ) = \info{X_1}{Y}$.

\Id:
We have $X \wedge Y \preceq X\vee Y$ by definition of $\wedge$ and $\vee$. Thus,
\begin{align*}
\Iw\!\left(X,Y : X\vee Y \right)
 &= \info{ X \wedge Y}{X\vee Y} \\
 &= \ent{ X \wedge Y} - \ent{X \wedge Y| X\vee Y} \\
 &= \ent{ X \wedge Y} \quad\mbox{by Lemma~\ref{lem:H}(a)} \\
 &= \infozero{X}{Y} \\
 &\not= \info{X}{Y} \; .
\end{align*}
\end{proof}

\begin{lem}\label{lem:Iwprop1}
The measure of intersection information $\Iw\!\left(X_1,\ldots,X_n \: Y \right)$ does not satisfy \Mone, \Sone, and \LPone.\end{lem}

\begin{proof}
\Mone:
A counterexample is provided in \textsc{ImperfectRdn} (\figref{fig:ImperfectRdn}), where $\Iw(X_1:Y)=0.99$ bits, yet $\Iw(X_1, Y:Y)=0$ bits.

\Sone: A counterexample.  We show $\Iwe{X,X}{Y} \not= \Iwe{X,Y}{X}$.
\begin{eqnarray*}
    \Iwe{X,X}{Y} - \Iwe{X,Y}{X} &=& \info{X}{Y} - \Iwe{X,Y}{X} \\
    &=& \info{X}{Y} - \info{X \wedge Y}{X} \\
    &=& \info{X}{Y} - \ent{X \wedge Y} - \ent{X \wedge Y|X} \\
    &=& \info{X}{Y} - \ent{X \wedge Y} \\
    &\not=& 0 \; .
\end{eqnarray*}

\LPone: This follows from not satisfying \LPzero.

\end{proof}

%----

\section{Miscellaneous Results}
\label{appendix:miscproofs}

\subsubsection*{Simplification of $\Iw^0$}

\begin{lem}\label{lem:Iw0}
We have  $\Iw^0\!\left(X_1, \ldots, X_n\!:\!Y\right) = \ent{X_1\wedge\cdots\wedge X_n\wedge Y}$.
\end{lem}
\begin{proof}
By definition,
\begin{align*}
\begin{split}
    \Iw^0\!\left(X_1, \ldots, X_n\!:\!Y\right) &\equiv \max_{ \Pr(Q|Y) } \infozero{Q}{Y} \\
    & \hspace{0.2in} \textnormal{subject to } Q \preceq X_i \ \forall i \in \{1, \ldots, n\} \\
%\end{split}\\
%\begin{split}
%\label{eq:Iw0satisfy}
%\hspace{1.25in}
&= \max_{\Pr(Q|Y) } \ent{Q \wedge Y} \\
    & \hspace{0.2in} \textnormal{subject to } Q \preceq X_i \ \forall i \in \{1, \ldots, n\} \\
\end{split}
\end{align*}
Let $Q$ be an arbitrary random variable satisfying the constraint $Q
\preceq X_i$  for $i=1,\ldots,n$.
Because $X_1\wedge\cdots\wedge X_n$ is the largest random
variable (in the sense of the partial order $\preceq$) that is
informationally poorer than $X_i$ for $i=1,\ldots,n$, we have
$Q\preceq X_1\wedge\cdots\wedge X_n$. By the property of $\wedge$ pointed out before, we
also have
$Q\wedge Y\preceq X_1\wedge\cdots\wedge X_n\wedge Y$.
By Lemma~\ref{lem:H}(b), this implies that
$\ent{Q\wedge Y} \leq \ent{X_1\wedge\cdots\wedge X_n\wedge Y}$.
Therefore, $\Iw^0\!\left(X_1, \ldots, X_n\!:\!Y\right) = \ent{X_1\wedge\cdots\wedge X_n\wedge Y}$.
\end{proof}

\subsubsection*{Simplification of $\Iw$}

\begin{lem}\label{lem:Iw}
We have
$\Iw\!\left(X_1, \ldots, X_n\!:\!Y\right) = \info{X_1\wedge\cdots\wedge X_n}{Y}$.
\end{lem}
\begin{proof}
By definition,
\begin{align*}
\begin{split}
    \Iw\!\left(X_1, \ldots, X_n\!:\!Y\right) &\equiv \max_{ \Pr(Q|Y) } \info{Q}{Y} \\
    & \hspace{0.2in} \textnormal{subject to } Q \preceq X_i \ \forall i \in \{1, \ldots, n\} \\
%\end{split}\\
%\begin{split}
%\label{eq:Iwsatisfy}
%\hspace{1.25in}
&= \ent{Y} - \min_{\Pr(Q|Y) } \ent{Y|Q} \\
    & \hspace{0.2in} \textnormal{subject to } Q \preceq X_i \ \forall i \in \{1, \ldots, n\} \\
\end{split}
\end{align*}
Let $Q$ be an arbitrary random variable satisfying the constraint $Q
\preceq X_i$  for $i=1,\ldots,n$.
Because $X_1\wedge\cdots\wedge X_n$ is the largest random
variable (in the sense of the partial order $\preceq$) that is
informationally poorer than $X_i$ for $i=1,\ldots,n$, we have
$Q\preceq X_1\wedge\cdots\wedge X_n$.
By Lemma~\ref{lem:H}(b), this implies that
$\ent{Y|Q} \geq \ent{Y|X_1\wedge\cdots\wedge X_n\wedge Y}$.
Therefore,
$\Iw\!\left(X_1, \ldots, X_n\!:\!Y\right) = \info{X_1\wedge\cdots\wedge X_n}{Y}$.
\end{proof}

\subsubsection*{Proof that $\Iwe{X_1, \ldots, X_n}{Y} \leq  \opI_{\min}\left( X_1, \ldots, X_n : Y \right)$}
%Need proof that,
%\begin{equation}
%    \Iww{X_1, \ldots, X_n}{Y} \leq \Iminn{X_1, \ldots, X_n}{Y} \; .
%\end{equation}

\begin{lem}\label{lem:IwleqImin}
We have $\Iwe{X_1, \ldots, X_n}{Y} \leq  \opI_{\min}\left( X_1, \ldots, X_n : Y \right)$
\end{lem}
\begin{proof}
    Starting from the definitions,
    \begin{align*}
        \Iwe{X_1, \ldots, X_n}{Y} &\equiv \info{X_1 \wedge \cdots \wedge X_n}{Y} \\
        &= \sum_{y} \Prob{y} \info{X_1 \wedge \cdots \wedge X_n}{y}  \\
        \Iminn{ X_1, \ldots, X_n}{Y} &\equiv \sum_{y} \Prob{y} \min_i \info{X_i}{y} \; .
    \end{align*}
For a particular state $y$, without loss of generality we define the
minimizing predictor $X_m$ by $X_m \equiv \argmin_{X_i}
\info{X_i}{y} $ and the common random variable $Q \equiv X_1 \wedge
\cdots \wedge X_n$.  It then remains to show that $\info{Q}{y} \leq \info{X_m}{y}$.

By definition of $\wedge$, we have $Q \preceq X_m$.  Hence,
\begin{align*}
    \info{X_m}{y}
    &= \ent{X_m} - \ent{X_m|Y=y} \\
    &\geq \ent{Q} - \ent{Q|Y=y}\quad\mbox{by Lemma~\ref{lem:H}(b)} \\
    &= \info{Q}{y} \; .
\end{align*}
\end{proof}

\subsubsection*{State-dependent zero-error information}
We define the state-dependent zero-error information, $\infozero{X}{Y=y}$ as,
\[
    \infozero{X}{Y=y} \equiv \log \frac{1}{\Prob{Q=q}} \; ,
\]
where the random variable $Q \equiv X \wedge Y$ and $\Prob{Q=q}$ is the probability of the connected component containing state $y \in Y$.  This entails that $\Prob{y} \leq \Prob{q} \leq 1$.  Similar to the state-dependent information, $\mathbb{E}_{Y} \infozero{X}{y}~=~\infozero{X}{Y}$, where $\mathbb{E}_{Y}$ is the expectation value over $Y$.
\begin{proof}
We define two functions $f$ and $g$:
\begin{itemize}
    \item $f : y \to q$ s.t. $\Prob{q|y}=1$ where $q \in Q$ and $y \in Y$.
    \item $g : q \to \{y_1, \ldots, y_k\}$ s.t. $\Prob{q|y_i}=1$ where $q \in Q$ and $y \in Y$.
\end{itemize}

Now we have,
\begin{equation*}
    \mathbb{E}_{Y} \infozero{X}{y} \equiv \sum_{y \in Y} \Prob{y} \log \frac{1}{\Prob{f(y)}} \; .
\end{equation*}

Since each $y$ is associated with exactly one $q$, we can reindex the $\sum_{y \in Y}$.  We then simplify to achieve the result.
\begin{eqnarray*}
\sum_{y \in Y} \Prob{y} \log \frac{1}{\Prob{f(y)}} &=& \sum_{q \in Q} \sum_{y \in g(q)} \Prob{y} \log \frac{1}{\Prob{f(y)}} \\
&=& \sum_{q \in Q} \sum_{y \in g(q)} \Prob{y} \log \frac{1}{\Prob{q}} = \sum_{q \in Q} \log \frac{1}{\Prob{q}} \sum_{y \in g(q)} \Prob{y} \\
&=& \sum_{q \in Q} \log \frac{1}{\Prob{q}} \Prob{q} = \sum_{q \in Q} \Prob{q} \log \frac{1}{\Prob{q}} \\
&=& \ent{Q} = \infozero{X}{Y} \; .
\end{eqnarray*}
\end{proof}

\clearpage
\section{Misc Figures}
\label{appendix:figs}

\begin{figure}[h!bt]
        \centering
        \begin{minipage}[c]{0.3\linewidth} \centering \subfloat[$\Prob{x_1, x_2, y}$]{ \begin{tabular}{ c | c c } \cmidrule(r){1-2}
$\ \, X_1 \, X_2$  &$Y$ \\
\cmidrule(r){1-2}
\bin{r r} & \bin{r} & \quad \nicefrac{1}{2}\\
\bin{R R} & \bin{R} & \quad \nicefrac{1}{2}\\
\cmidrule(r){1-2}
\end{tabular}
\label{fig:RDNa} }
\end{minipage} \begin{minipage}[c]{0.33\linewidth} \centering
        \subfloat[circuit diagram]{ \includegraphics[width=1.9in]{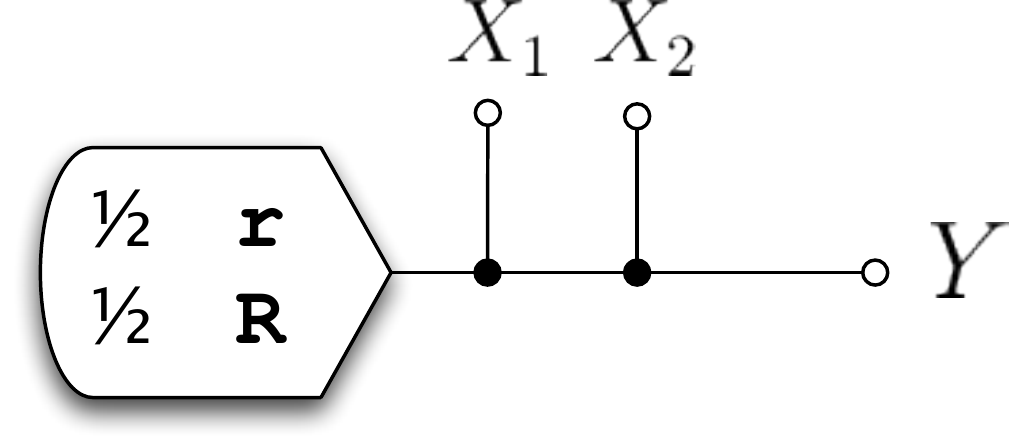} }
        \end{minipage}
        \begin{minipage}[c]{0.33\linewidth} \centering
        \begin{align*}
        \info{X_1 X_2}{Y} &= 1 \\
        \info{X_1}{Y} &= 1 \\
        \info{X_2}{Y} &= 1 \\
        \addlinespace
    \Iminn{X_1,X_2}{Y} &= 1  \\
    \Iwe{X_1,X_2}{Y} &= 1
        \end{align*}
        \end{minipage}
        \\[1.5em]
        \begin{minipage}[c]{0.33\linewidth} \centering
        \subfloat[$\opI_{\min}$]{ \includegraphics[width=1.4in]{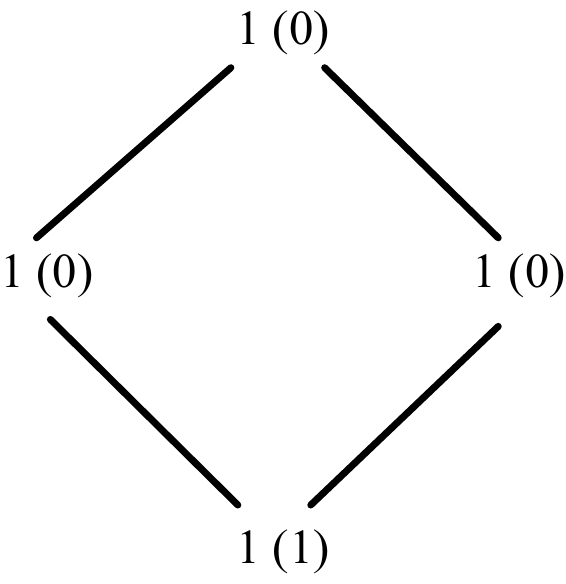} \label{fig:cs1} }
    \end{minipage}
        \begin{minipage}[c]{0.33\linewidth} \centering
        \subfloat[$\Iw$ and $\Iw^0$]{ \includegraphics[width=1.4in]{PID2-RDN.pdf} \label{fig:cs2} }
    \end{minipage}
        \caption{Example \textsc{Rdn}. In this example $\opI_{\min}$ and $\Iw$ reach the same answer yet diverge drastically for example \textsc{ImperfectRdn}.}
        \label{fig:RDN}
\end{figure}
